# Supplementary material for: The Expressive Power of Word Embeddings
Source: arXiv:1301.3226 source file (2013-05-29)
Supplement: Supplementary file 1 [file appendix.tex]

\newpage
\section{Appendix}
\subsection{PCA Table}
\begin{table}[!htb]
\begin{scriptsize}
\begin{center}
\begin{tabular}{|l|l|l|l|l|l|l|l|l|}
\hline
\ Training method & SENNA & \multicolumn{2}{|c|}{HLBL embedding} & \multicolumn{4}{|c|}{Turian's embedding} & SBU \\
\ Dimension & 50 & \multicolumn{1}{l}{50} & 100 & \multicolumn{1}{l}{25} & \multicolumn{1}{l}{50} & \multicolumn{1}{l}{100} & 200 & 64\\
\hline
\ PCA components=5 & 76.92\% & 58.4\% & 61.96\% & 45.88\% & 57.76\% & 62.80\% & 66.46\% & 69.37\% \\
\hline
\ PCA components=10 & 83.78\% & 70.69\% & 71.14\% & 70.21\% & 76.17\% & 72.36\% & 76.37\% & 84.65\% \\
\hline
\ PCA components=15 & 86.02\% & 74.99\% & 76.73\% & 77.34\% & 75.49\% & 77.23\% & 74.97\% & 83.17\% \\
\hline
\ PCA components=20 & 85.30\% & 78.92\% & 74.39\% & 78.78\% & 78.07\% & 75.83\% & 78.78\% & 85.78\% \\
\hline
\ PCA components=25 & 87.58\% & 79.83\% & 78.23\% & N/A & 79.26\% & 79.46\% & 75.32\% & 87.92\% \\
\hline
\ PCA components=50 & N/A & N/A & 79.19\% & N/A & N/A & 80.00\% & 79.31\% & 87.76\% \\
\hline
\ PCA components=100 & N/A & N/A & N/A & N/A & N/A & N/A & 77.60\% & N/A \\
\hline
\end{tabular}

\begin{tabular}{|l|l|l|l|l|l|l|l|l|}
\hline
\ Training method & SENNA & \multicolumn{2}{|c|}{HLBL embedding} & \multicolumn{4}{|c|}{Turian's embedding} & SBU \\
\ Dimension & 50 & \multicolumn{1}{l}{50} & 100 & \multicolumn{1}{l}{25} & \multicolumn{1}{l}{50} & \multicolumn{1}{l}{100} & 200 & 64\\
\hline
\ PCA components=5 & 81.01\% & 67.02\% & 70.19\% & 65.23\% & 69.22\% & 71.30\% & 72.71\% & 75.43\% \\
\hline
\ PCA components=10 & 86.62\% & 75.55\% & 76.99\% & 76.06\% & 79.97\% & 78.88\% & 81.06\% & 87.90\% \\
\hline
\ PCA components=15 & 88.40\% & 79.32\% & 81.25\% & 80.92\% & 80.08\% & 81.45\% & 80.01\% & 86.27\% \\
\hline
\ PCA components=20 & 87.79\% & 82.7\% & 79.92\% & 81.81\% & 81.88\% & 80.54\% & 82.37\% & 88.3\% \\
\hline
\ PCA components=25 & 89.84\% & 83.37\% & 82.52\% & N/A & 83.07\% & 83.32\% & 80.89\% & 90.21\% \\
\hline
\ PCA components=50 & N/A & N/A & 83.69\% & N/A & N/A & 83.85\% & 82.55\% & 90.13\% \\
\hline
\ PCA components=100 & N/A & N/A & N/A & N/A & N/A & N/A & 81.73\% & N/A \\
\hline
\end{tabular}
\end{center}
\end{scriptsize}
\caption{F1 score (top) and accuracy (bottom) after doing PCA, SVM RBF kernel on sentiment problem}
\label{pca1}
\end{table}

\subsection{Dimension Reduction Tasks}
\begin{figure}
\centering
\centering
\begin{subfigure}
    \centering
    \includegraphics{f1_diff_linear_regression.eps}
\end{subfigure}
\begin{subfigure}
    \centering
    \includegraphics{Acc_diff_linear_regression.eps}
\end{subfigure}
\caption{F1 score (top) and Accuracy (bottom) difference, linear regression model}
\end{figure}
   
\begin{figure}
\centering
\begin{subfigure}
    \centering
    \includegraphics{f1_diff_svm_linear.eps}
\end{subfigure}
\begin{subfigure}
    \centering
    \includegraphics{Acc_diff_svm_linear.eps}
\end{subfigure}
\caption{F1 score (top) and Accuracy (bottom) difference, SVM linear kernel model}
\end{figure}

\begin{figure}
\centering
\begin{subfigure}
    \centering
    \includegraphics{f1_diff_svm_rbf.eps}
\end{subfigure}
\begin{subfigure}
    \centering
    \includegraphics{Acc_diff_svm_rbf.eps}
\end{subfigure}
\caption{F1 score (top) and Accuracy (bottom) difference, SVM RBF kernel model}
\end{figure}
